# Supplementary material for: Explainable Data Imputation using Constraints
Source: arXiv:2205.04731 source file (2022-05-10)
Supplement: Supplementary file 1 [file appendix.tex]

\section{More Results}

% \begin{figure*}
% \centering
% \subcaptionbox{Avg. NRMSE for all numerical columns}{\includegraphics[width=0.50\textwidth]{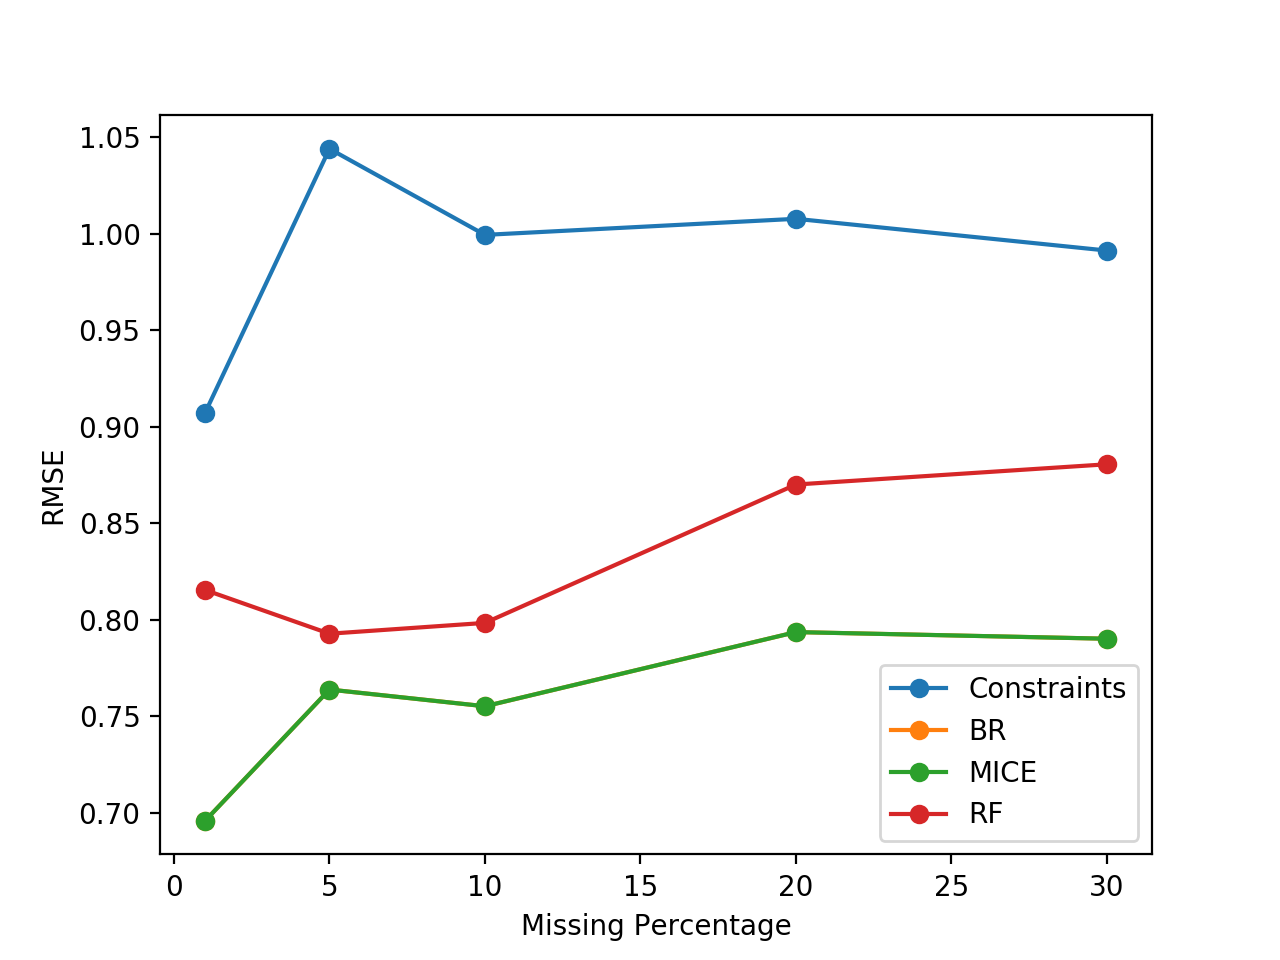}}%
% \subcaptionbox{Columnwise NRMSE}{\includegraphics[width=0.50\textwidth]{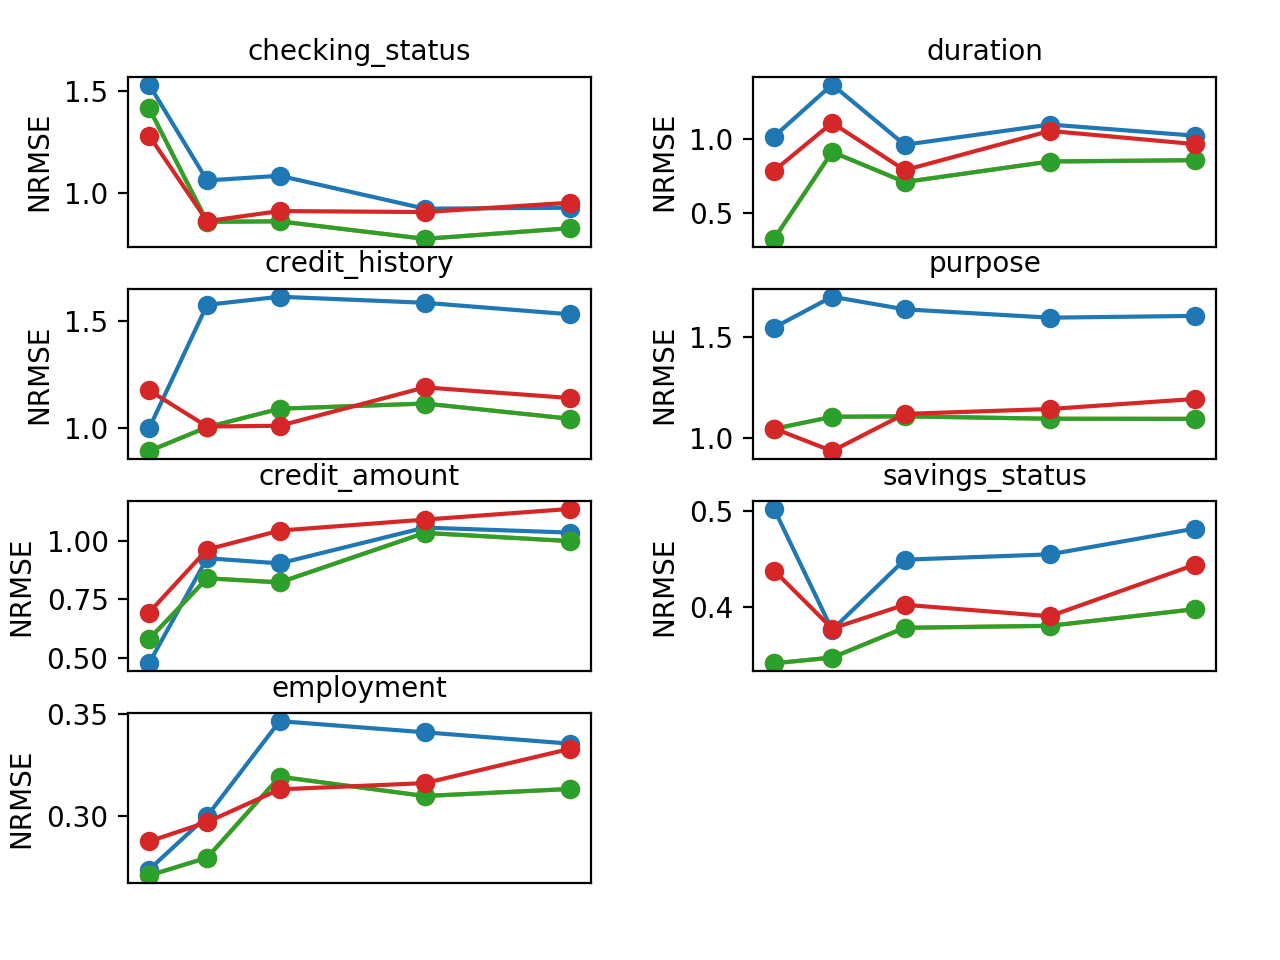}}%
% \caption{Numerical Imputation results on credit dataset from openml.}
% \label{fig:num_results_credit}
% \end{figure*}
%\subsection{Categorical Imputation}

\begin{figure*}
\centering
\subcaptionbox{}{\includegraphics[width=0.30\textwidth]{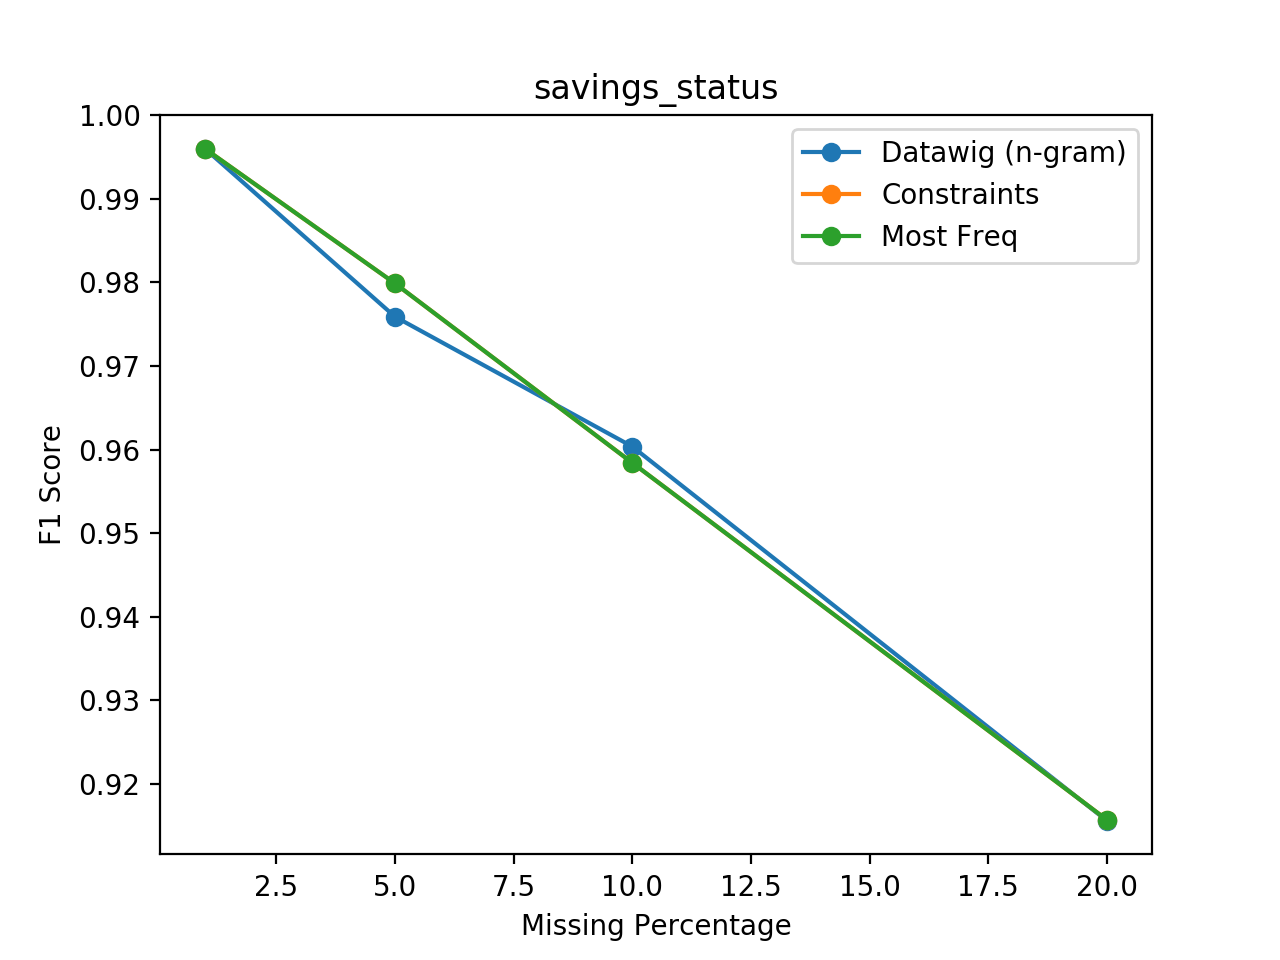}}%
\subcaptionbox{}{\includegraphics[width=0.30\textwidth]{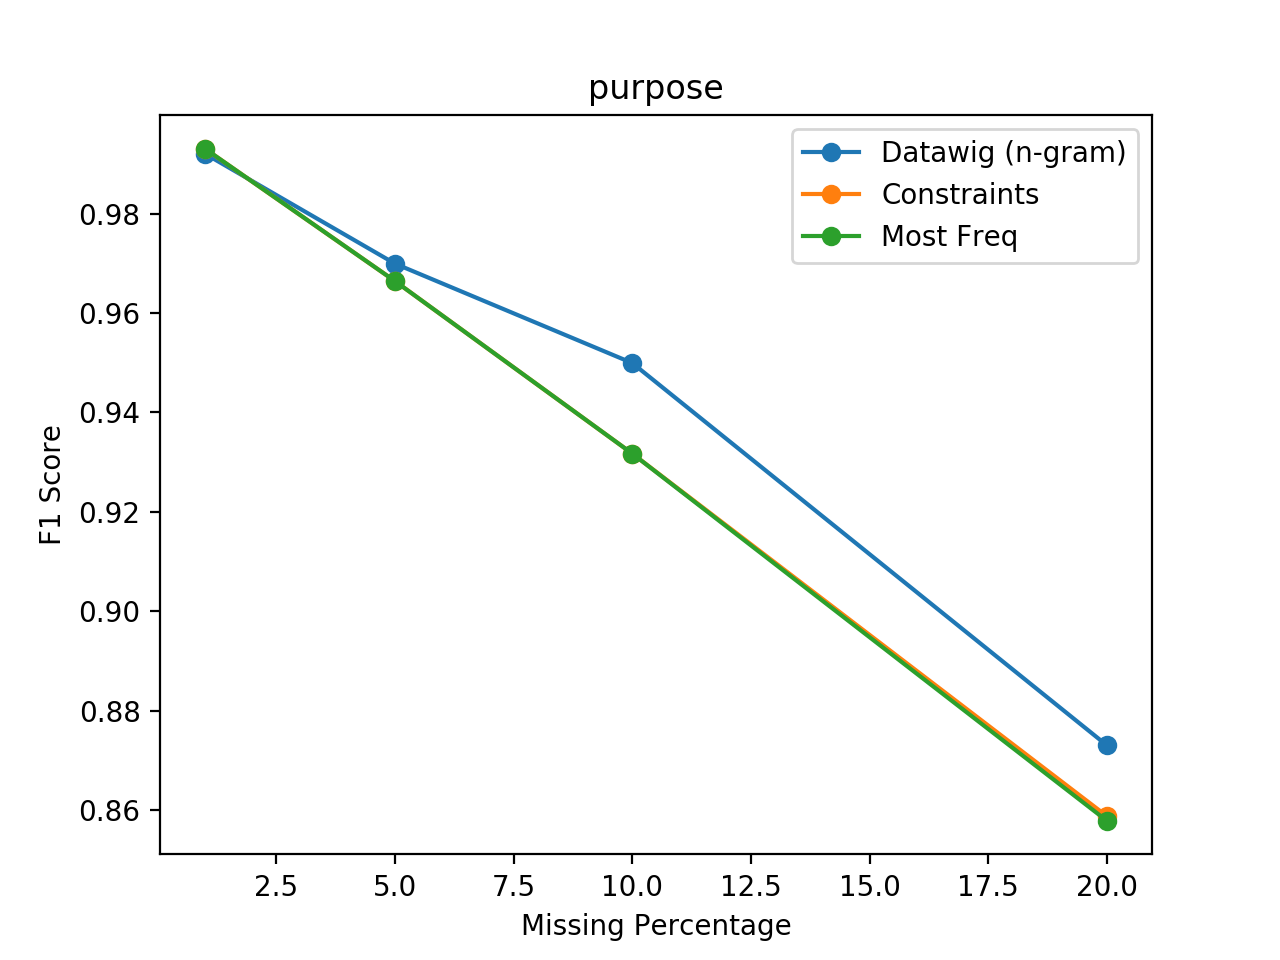}}%
\subcaptionbox{}{\includegraphics[width=0.30\textwidth]{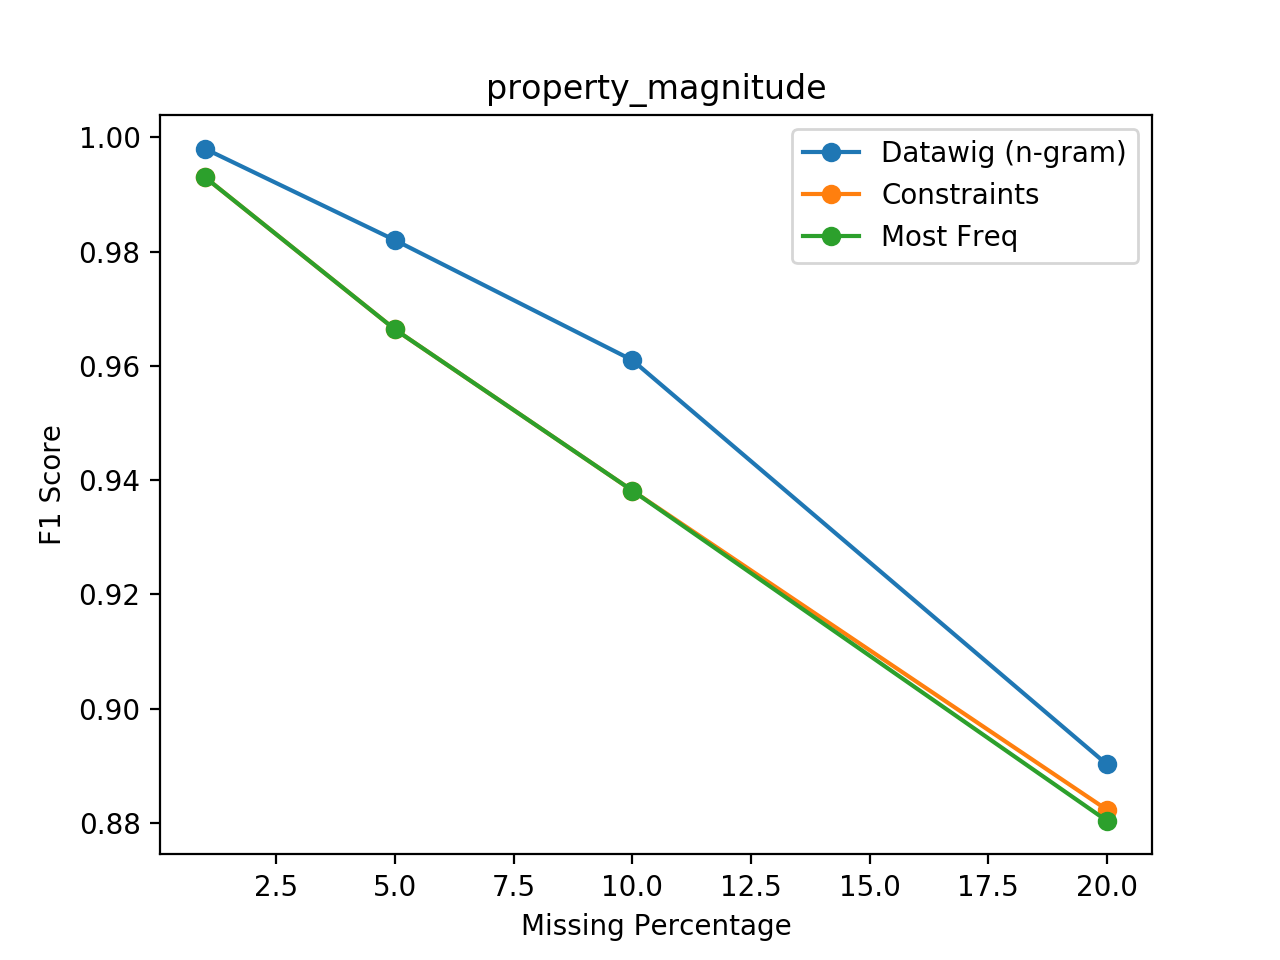}}%
\par
\subcaptionbox{}{\includegraphics[width=0.30\textwidth]{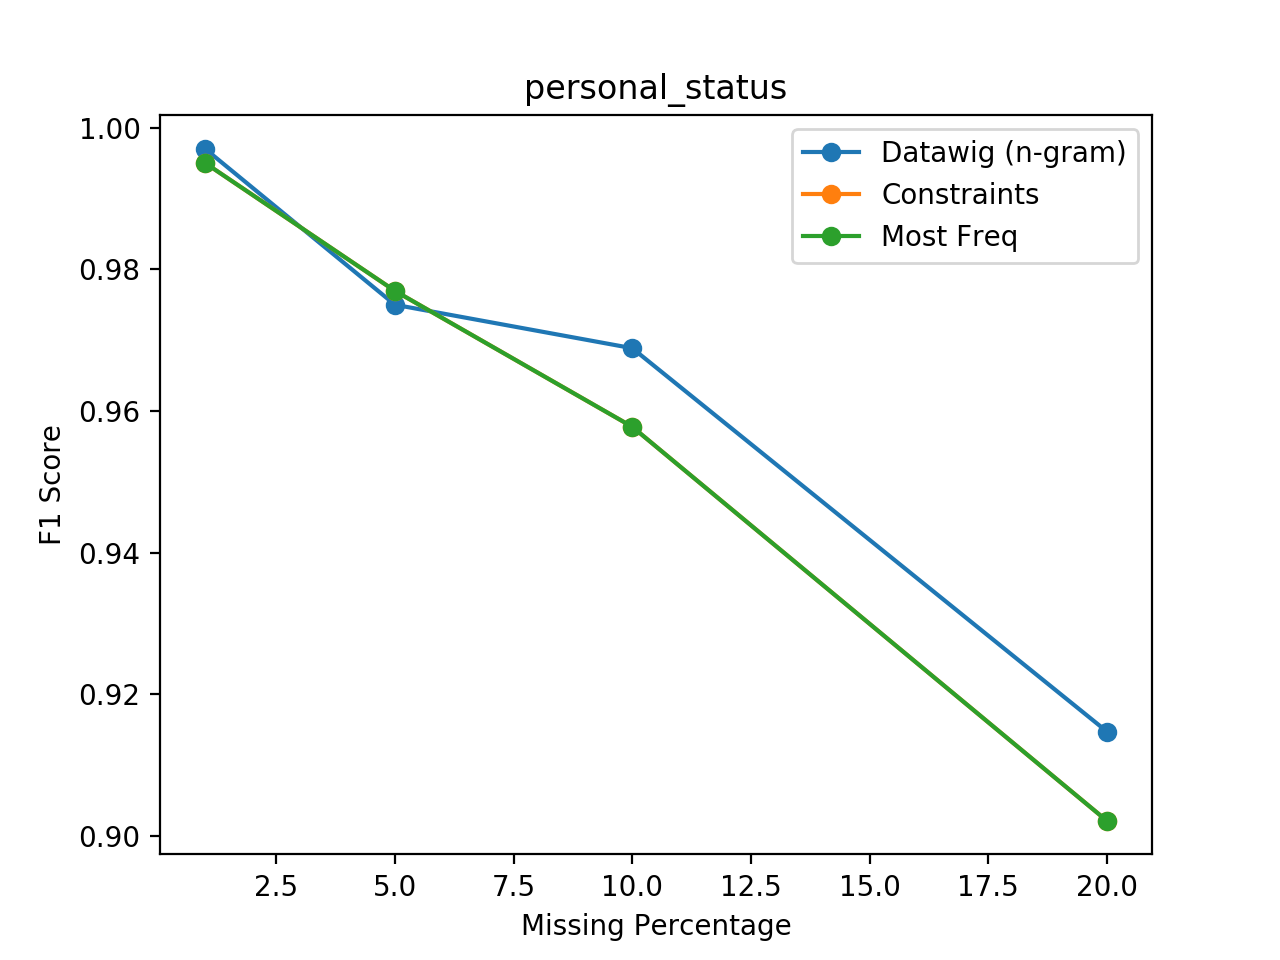}}%
\subcaptionbox{}{\includegraphics[width=0.30\textwidth]{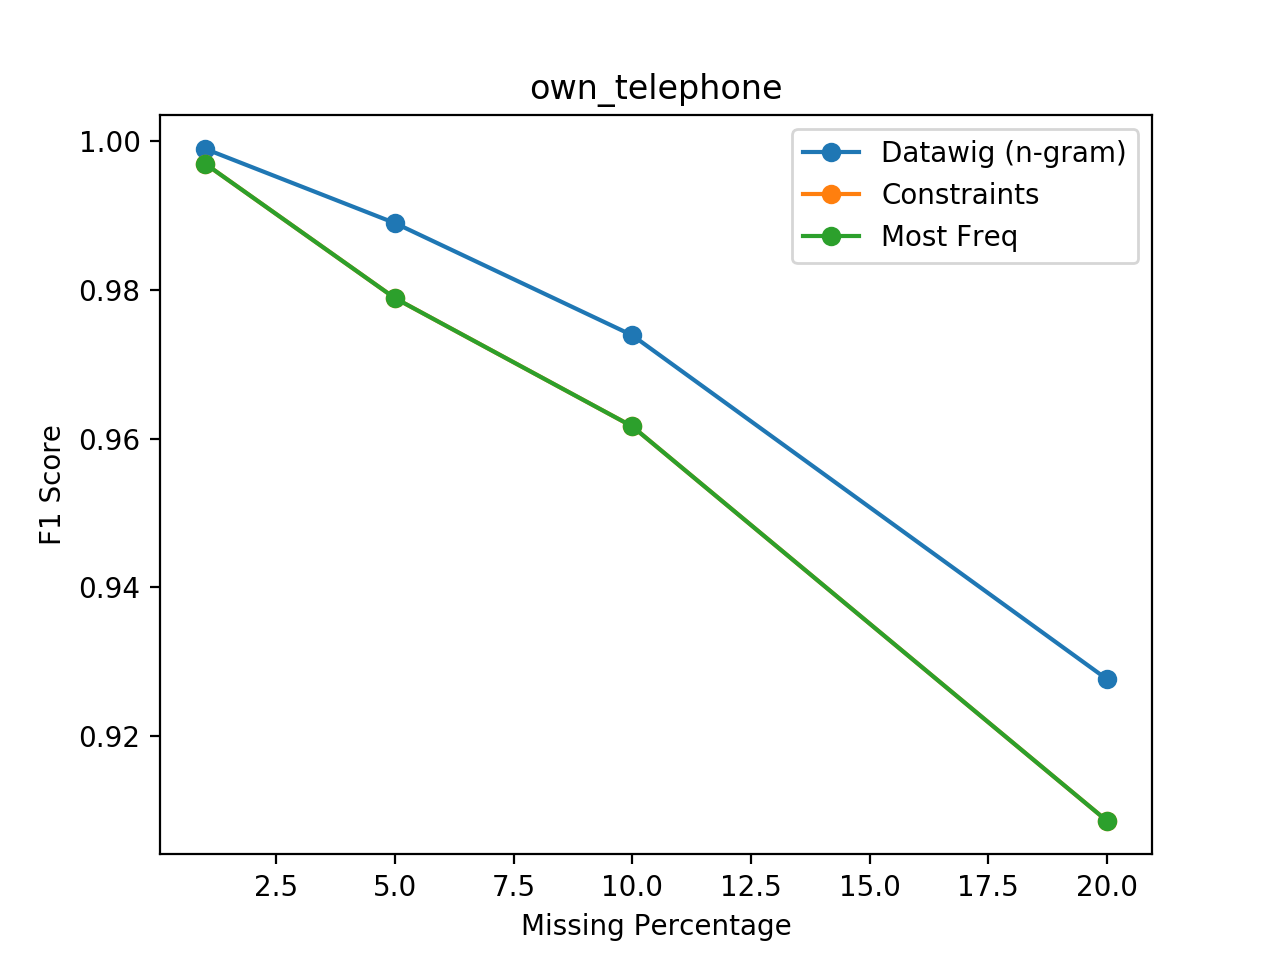}}%
\subcaptionbox{}{\includegraphics[width=0.30\textwidth]{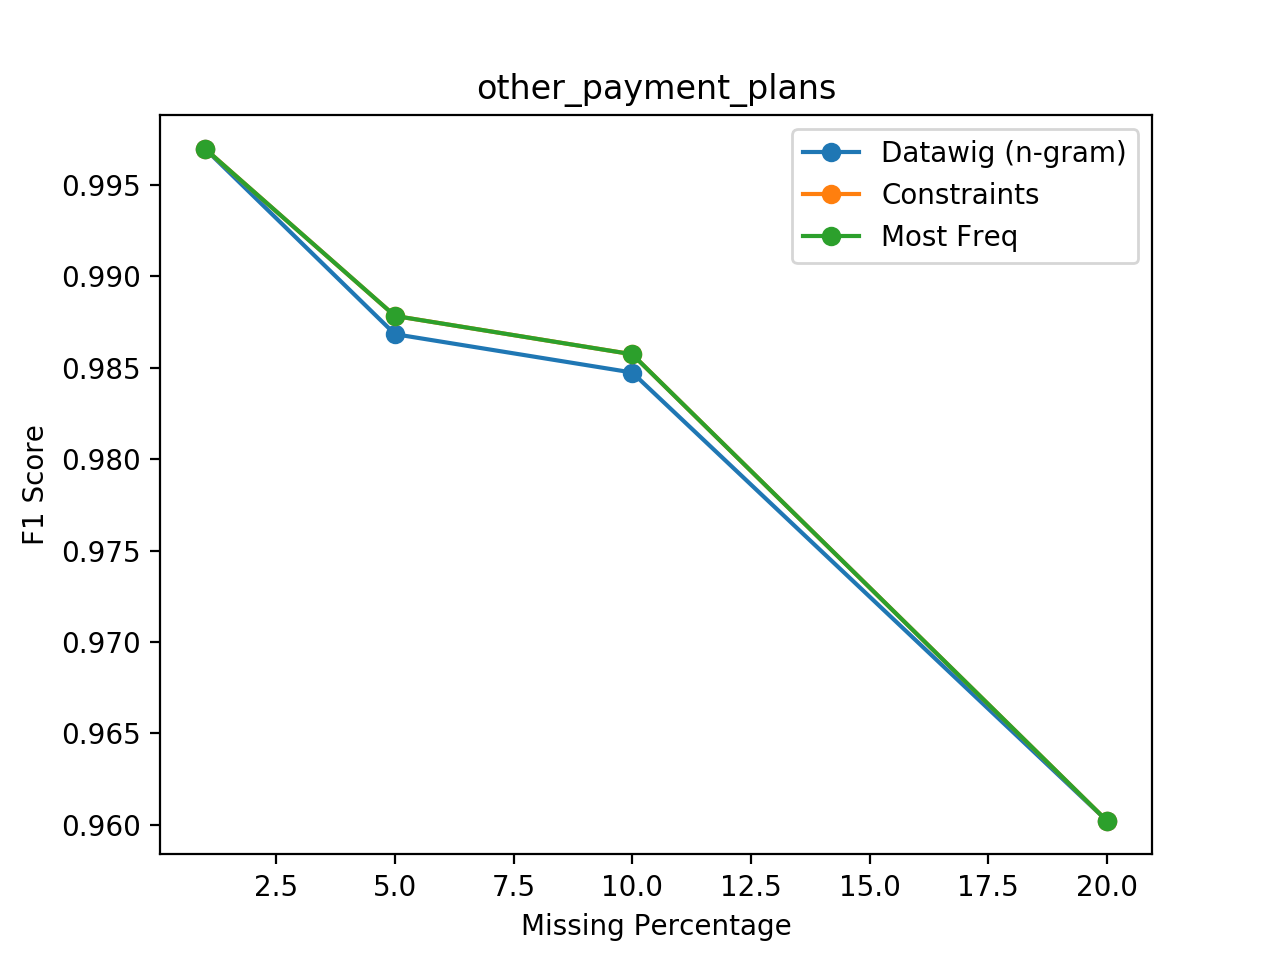}}%
\par
\subcaptionbox{}{\includegraphics[width=0.30\textwidth]{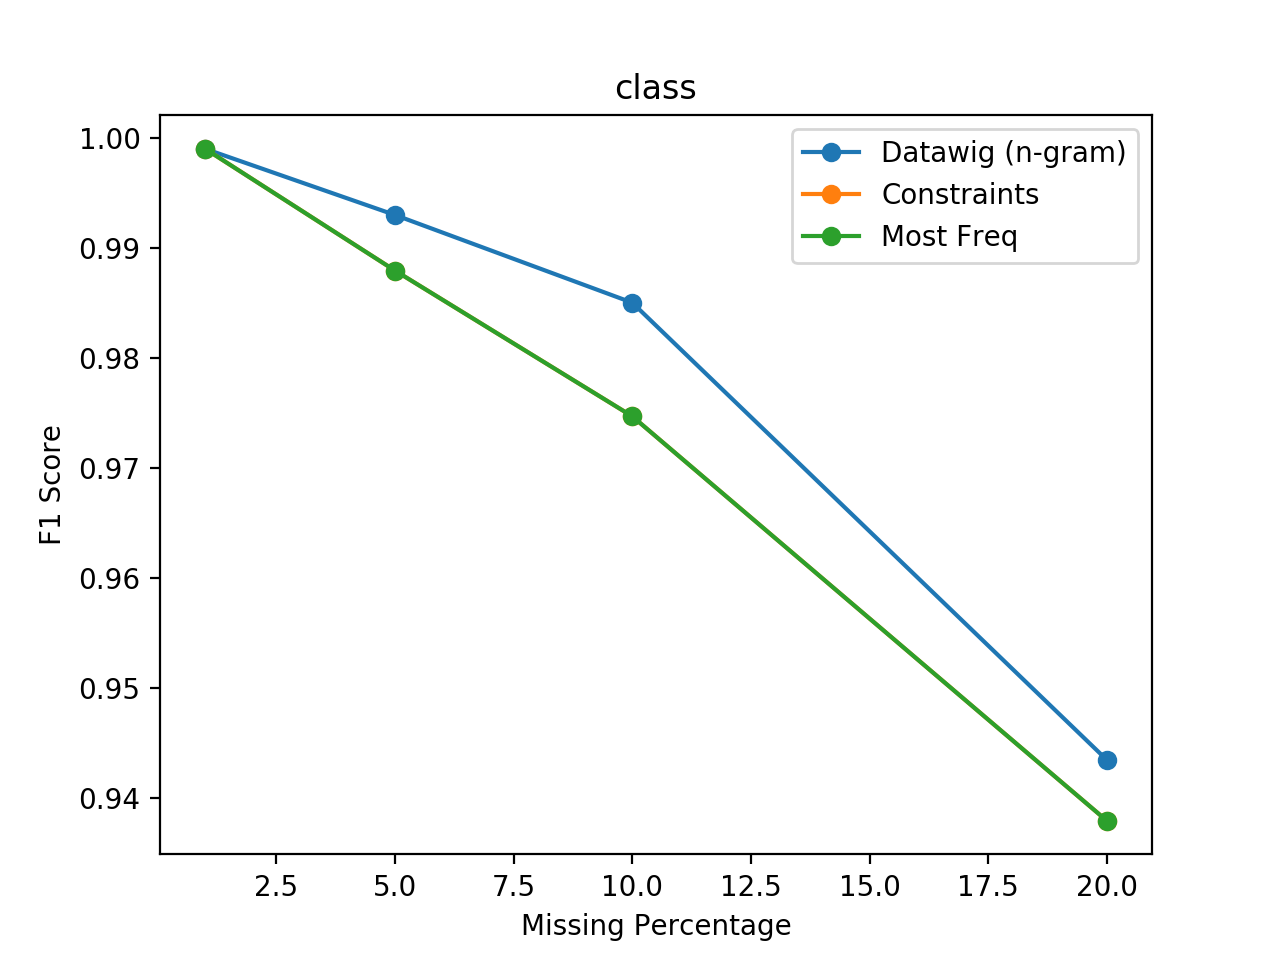}}%
\subcaptionbox{)}{\includegraphics[width=0.30\textwidth]{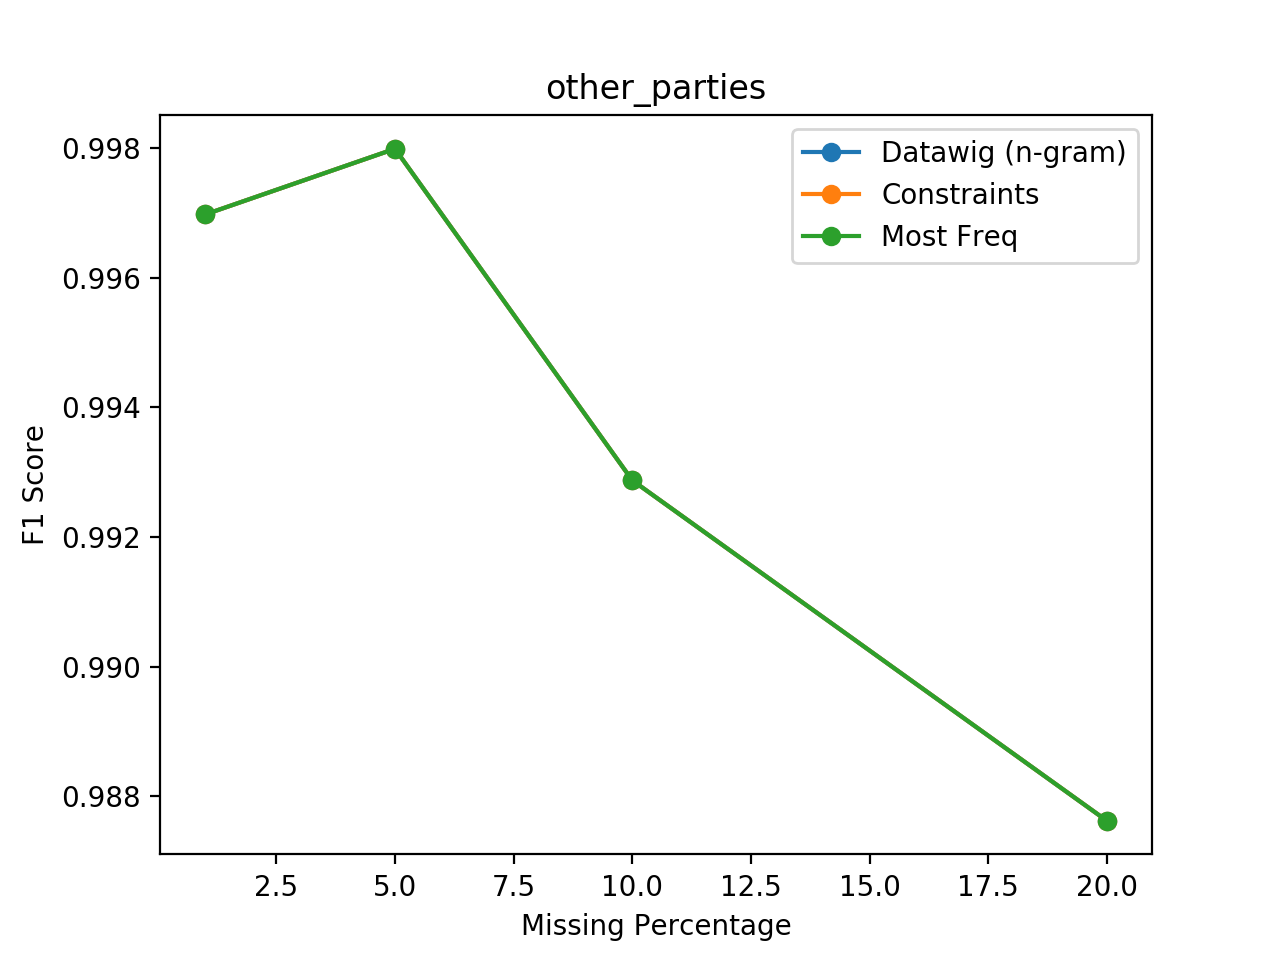}}%
\subcaptionbox{}{\includegraphics[width=0.30\textwidth]{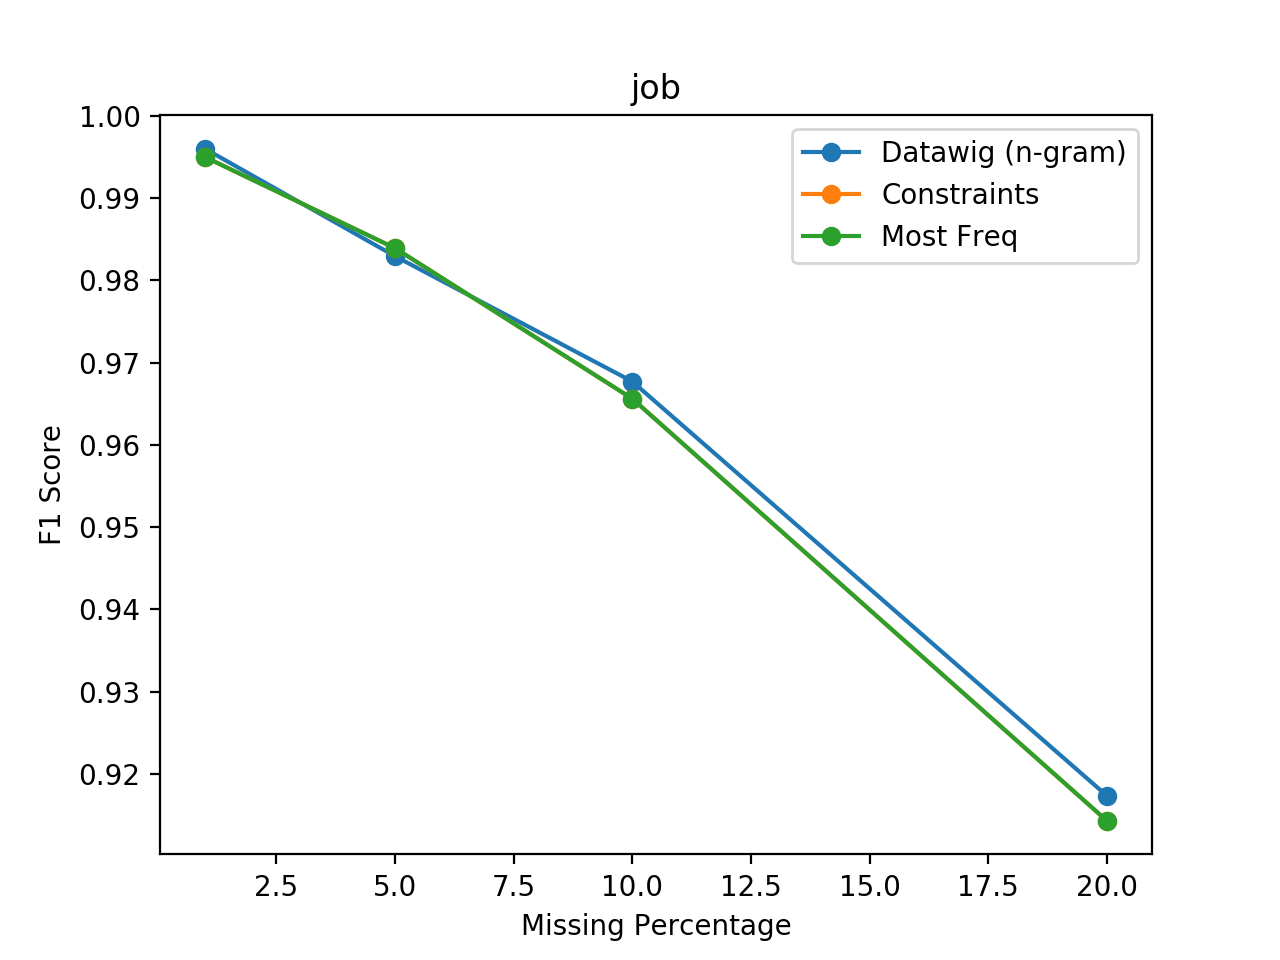}}%
\caption{Categorical Imputation results on credit dataset from openml.}
%\label{fig:cat_results}
\end{figure*}
